# Supplementary material for: Bulk Electronic Structure of Ni2MnGa studied by Density Functional Theory and Hard X-ray Photoelectron Spectroscopy
Source: arXiv:2304.04992 source file (2023-08-31)
Supplement: Supplementary file 1 [file Supplementary_dft_haxpes_nmg_R1_final.pdf]

# Supplementary Material for Bulk Electronic Structure of $Ni_2MnGa$ studied by Density Functional Theory and Hard X-ray Photoemission Spectroscopy

Joydipto Bhattacharya[1,2,†], Pampa Sadhukhan[3,†], Shuvam Sarkar[3], Vipin Kumar Singh[3], Andrei Gloskovskii[4], Sudipta Roy Barman[1], and Aparna Chakrabarti[1,2]

[1] *Homi Bhabha National Institute, Training School Complex, Anushakti Nagar, Mumbai 400094, India*
[2] *Raja Ramanna Centre for Advanced Technology, Indore 452013, India*
[3] *UGC-DAE Consortium for Scientific Research, Khandwa Road, Indore 452001, India and*
[4] *Deutsches Elektronen-Synchrotron DESY, Notkestrasse 85, D-22607 Hamburg, Germany*

**The supplementary material contains the Methodology and four notes (Note A-D), six tables (Table S1-S6), and thirteen figures (Figs. S1-S13).**

## I. METHODOLOGY

### I.1. Density functional theory

Electronic structure calculations have been performed for the austenite and martensite phases of $Ni_2MnGa$ using density functional theory employing Vienna Ab Initio Simulation Package (VASP) [1]. Generalized gradient approximation (GGA) over local density approximation was used for the exchange-correlation functional [2]. For the austenite phase, we have considered the experimentally determined $L2_1$ structure with the lattice constants: $a = b = c = 5.82$ Å [3]. In case of the martensite phase, the calculations were carried out using 7-fold orthorhombic unit cells obtained from experiments, as reported in the literature [4–7]. These structures contain total of 56 atoms i.e., 28 Ni, 14 Mn and 14 Ga atoms. The calculations were performed considering the experimentally determined structures without any structure optimization. We also consider another well-known theoretical model (14M NT) for the martensite phase. For this model structure (NTN-K) with 56 atoms, full geometry optimization has been performed. Fig. S1 compares the different structures and Tables S1-S5 contain the relevant structural information.

The density of states (DOS) calculations have been carried out for both the austenite and martensite phases of $Ni_2MnGa$. For the self-consistent-field (SCF) calculations, we have set the energy convergence criteria to $10^{-6}$ eV and the force convergence criterion was set to $10^{-2}$ eV/Å. A high kinetic energy cutoff of 500 eV was used for all calculations to address the small energy difference between different modulated structural phases. The Brillouin zone was sampled by the Monkhorst-Pack [8] $k$-points generation scheme, where a 15×15×15 $k$-mesh grid was used for the austenite phase and a 17×5×15 $k$-mesh grid was used for rest of the martensite phases. For the calculations of DOS, much larger $k$-mesh has been used for both the austenite and martensite structures.

### I.2. HAXPES experiment

The HAXPES measurements were performed at the P09 beamline in PETRA III synchrotron center, Germany [9]. Photons were incident on the sample at a grazing angle (10°) and the photoelectrons were detected at normal emission angle. $Ni_2MnGa$ single crystal was grown by the Bridgman technique [10]. The stoichiometry of the bulk composition was confirmed by wavelength dispersive x-ray spectroscopy to be $Ni_{2.03}MnGa_{0.96}$ [11, 12]. From heat flow data for the bulk crystal, the martensite start temperature ($M_s$) and the austenite start temperature were determined to be 206.5 K and 215.7 K, respectively [11, 12]. The (100) surface of this $Ni_2MnGa$ single crystal was studied by low energy electron diffraction and low energy photoemission spectroscopy in Refs. [11–13]. Although HAXPES is bulk sensitive with large inelastic mean free path, the specimen studied is prone to oxidation on exposure to ambient conditions. Hence, this was fractured under ultra-high vacuum at $2\times10^{-8}$ mbar pressure to expose fresh surface and this was immediately transferred into the analysis chamber at a base pressure of $2\times10^{-9}$ mbar. The instrumental resolution [including both source and analyzer contributions] obtained from the Fermi edge of Au that was in electrical contact with the specimen is 140 meV.

### I.3. VB calculation

The calculated VB spectra, for comparison with the HAXPES results, were obtained from the partial density of states (PDOS), as discussed in Ref. [14]. All the atom and angular momentum projected PDOS were multiplied by the corresponding photoemission cross-sections per electron [15] [$\sigma_i = \sigma_{tot}/n$, where $n$ is the electron occupancy of the corresponding shell] and added. This then was multiplied by a Fermi function, which was convoluted with a Gaussian function representing the instrumental broadening and a Lorentzian function of increasing width with binding energy representing an energy dependent lifetime broadening [16]. An inelastic background [17] was added to simulate the experimental background.

## II. NOTE A

The results of electronic structure of cubic phase of $Ni_2MnGa$ are presented in Fig. S2(a). At $E_F$, a relatively large DOS [with 1.11 states/eV-fu at $E_F$] is observed that has contribution mainly from minority spin of Ni 3$d$ states. We find that the DOS is about 10 eV wide in the occupied region below $E_F$. Various prominent features are seen in this range of VB at about ($a_1$)-0.21 eV, ($b_1$)-1.1 eV, ($c_1$)-1.7 eV, ($d_1$)-3.1 eV and we find some relatively broader peaks at about ($e_1$)-5.3 eV and ($f_1$)-7.3 eV. Notably, features ($b_1$) and ($c_1$) put together yield a somewhat broad peak in the range of -1 to -2 eV, with the largest intensity around -1.7 eV. In order to explain the origin of these features, we analyze the calculated PDOS of $Ni_2MnGa$ in the austenite phase with $L2_1$ structure [Fig. S2(a) and Fig. 1 of main text]. We see that the VB has significant contributions from Ni 3$d$ and Mn 3$d$ hybridized states and a small contribution from the Ni 4$s$, Ga 4$s$ and 4$p$ states over a wide range from $E_F$ to -10 eV. The feature $a_1$ corresponds predominantly to the Ni 3$d$ down states, hybridized with Ga and also Mn states, as observed in the literature [18]. Features $b_1$ and $c_1$ have major contributions from the Ni 3$d$ states in both the spin channels and Mn 3$d$ majority spin states; the former shows that a significant contribution is from the Mn atom. The peak at -3.16 eV can be almost entirely assigned to the Ni 3$d$ [both up and down spin] and Mn 3$d$ [up spin] hybridized states. Spin-polarized PDOS of Mn consists of majority states of Mn 3$d$ below $E_F$, showing two peaks at -1.2 eV and -3.1 eV, whereas the minority states lie above $E_F$ with a peak at 1.5 eV, which is in agreement with the literature. This well separated majority and minority states of Mn 3$d$ states indicate a large exchange splitting. This is manifested by the large partial moment of Mn of 3.3 $\mu_B$. These results agree well with our previous DFT calculations using the full potential linearized augmented plane wave (FPLAPW) method [19].

## III. NOTE B

*Structure MDL-B* – For the structure given by Brown *et al.* [4], we analyze Figs. S2(b) and S5. A hump around $E_F$ has been seen, in the down spin channel, unlike any of the other martensite cases, which has clear contribution from Ni atoms. In the respective up spin case, we notice less clear and almost equal contributions from the Mn and Ni atoms. We see a small peak-like feature around -0.4 eV which shows contributions from different atoms as seen in case of the hump at $E_F$. A clear peak at -0.95 eV arises due to the up spin states of both Mn and Ni atoms. This merges with two bigger peaks and the three put together form a broad three peak kind of structure. While the one at -1.3 eV is mainly due to Ni down spin states, the one around -1.8 eV can be associated with the up spin states of Ni atoms. A broad peak, centered around -3.5 eV, spans the range of slightly less than -3 to slightly less than -4 eV. In this range, where the down spin contributions are from Ni and Ga, the up spin contributions come from Ni and Mn atoms. The contributions for the higher BE features around -5.5 and -7.5 eV are same as the NTN-K case.

*Structures MDL-R and MDL-S* - The TDOS and PDOS related to the structures given by Righi *et al.* and Singh *et al.* are depicted in Figs. S2(c,d), S6, and S7. The features and the peak positions as well as relative intensities of the TDOS and PDOS have been found to be very close for these two structures, except the dip below -0.6 eV is slightly more clear for the MDL-S case. This similarity in the electronic structures of MDL-R and MDL-S corroborates with the structural data: the lattice parameters and fractional atomic coordinates for these two structures are very similar to each other, as is clear from Tables S3 and S4. Therefore, we discuss here the detailed DOS results for one of these structure, which is given by Singh *et al.*

From Fig. S2(d), we find that just above $E_F$, a somewhat sharp peak shows up which consists of mainly down spin states of Ni atom. Signature of up spin states of Ni, Mn and Ga atoms, and down spin states of Mn and Ga atoms are also there. At about -0.6 eV ($a_2$), a peak mainly arising from Ni down spin is prominent. Rest [Ni, Mn and Ga up and Mn and Ga down spin] has small contributions as well. A hump in the up spin channel at -1 eV is seen which is due to Ni atom, Mn atoms also are present [toward higher BE]. Between -1 to -3 eV a broad peak with a multi-peak structure can be seen. At about -1.5 eV ($b_2$), a peak corresponding to the up spin has both Ni and Mn contribution. At an energy close to that [-1.65 eV], the down spin states of Ni atom dominate. States in the range of about -1.75 to -2.75 eV mainly correspond to the up and down spin states of Ni atom. A double peak type structure is observed in up and down spin channels in the range of about -3 to -3.6 eV. Just above -3 eV, Ni and Ga down spin states are hybridized and overall from -3 to -3.6 eV, hybridized Ni and Mn up spin states dominate ($c_2$). Just below -4 eV, a hump is observed, which consists of hybridized up spin states of all Ni, Mn and Ga atoms; it has small down spin contribution from Ni and Ga atoms as well. Two relatively broader peaks at about -5.5 eV ($d_2$) and -7.5 eV ($e_2$) have also been observed; while the former has contribution from all the three atoms, the latter is dominated by the Ga states as in other cases.

*NTN-K* - A well-studied theoretical model for the martensite phase of $Ni_2MnGa$ is the 14M nanotwin structure [20, 21]. The details of the same are presented in Fig. S1(e) as well as Table S5. The spin-polarized density of states [Fig. S2(e)] has been calculated for this structure, following full geometry optimization of the structure. Fig. S8 contains the atom-projected total DOS (top panel), which has been utilized to calculate the VB spectrum (bottom panel) corresponding to this structure. From Fig. S2(e), a somewhat shoulder-like

feature around -0.5 eV can be seen. While in the down spin channel, it consists of Ni states, in the up spin case, it is due to both Ni and Mn atoms. A clear peak ($a_3$) is seen around -0.86 eV in the up spin channel, which is mainly due to the Ni atoms and a less prominent contribution comes from Mn atoms. A prominent peak ($b_3$) is seen in the range of -1 to -2 eV, centered around -1.4 eV [see Fig. S2(e)], which has contribution from both the spin channels. In case of up spin channel, it can be mainly assigned to Ni atoms, with some contribution coming from Mn atoms but in case of down spin, it is almost entirely due to the Ni atoms. In the TDOS, a clear two peak type structure ($c_3$ and $d_3$) is seen in the range -2 to -3 eV. Near to -2 eV ($c_3$), the peak is dominated by down spin states of Ni atoms only. Near to -3 eV ($d_3$), contribution in the up spin channel is mainly from Ni atoms, but considerable contribution of Mn atoms is seen as well on the higher binding energy (BE) side compared to Ni. Down spin states of Ni atoms are also found to be present. A broad peak-like feature centered at about -3.5 eV ($e_3$) is dominated by Ni and Mn atoms (Ni atom) in the up (down) spin channel. A hump-like feature due to a hybridized state of all of the Ni, Mn and Ga atoms is found at -3.8 eV. We find that two less intense and broad peaks appear at about -5.5 eV ($f_3$) and -7.5 eV ($g_3$). The features $f_3$ ($g_3$) consists of states from all the three atoms [primarily Ga states] as can be seen from the VB spectra presented in the bottom panel of Fig. S8.

Overall, for all the four structures, we find that the Ni 3$d$ states clearly contribute to the DOS close to the $E_F$ [primarily dominated by the minority states] as well as the whole VB spectrum, as shown by earlier first-principles calculations for the cubic and non-modulated tetragonal phases [22, 23]. Few of the features in the higher BE have dominant contributions from the Mn 3$d$ states, while Ga 4$s$ and 4$p$ states contribute significantly to the density of states, in much higher BE side [below -7 eV].

## IV. NOTE C

*Results of GGA+U calculations* – Although the agreement between HAXPES and DFT-GGA calculations using the experimentally reported modulated structures MDL-S [6] and MDL-R [5] is already very good, the effect of the Coulomb interaction parameter $U$ on the modulated martensite phase is an interesting question. Relatively large values of $U$ have been suggested in some recent theoretical studies, for example, $U_{\mathrm{Mn}} = 3.93$ eV [26], $U_{\mathrm{Mn}}= U_{\mathrm{Ni}}=$ 3eV [24] and $U_{\mathrm{Mn}}=$ 1.8 eV [25]. We have performed the DFT calculations using GGA+U exchange correlation functional for the modulated CDW phase (MDL-S structure) with $0.5\leq U_{\mathrm{Mn}}\leq 3$ eV, and also additionally for $U_{\mathrm{Ni}}$ with $0.5\leq U_{\mathrm{Ni}}\leq 3$ eV. In order to estimate the value of $U$ for $Ni_2MnGa$, we compare (a) the theoretical VB including $U$ with the experimental valence band and (b) the experimental total saturation magnetic moment in the martensite phase with that obtained from theory. A comparison with the DFT VB calculated with $U_{\mathrm{Mn}}=$ 0.5 eV with the experimental VB marginally improves the agreement for the most intense feature **B** (see the region highlighted by a blue dashed oval in Fig. S9 of SM). The position of feature **B** shifts by about 0.1 eV towards higher binding energy for $U_{\mathrm{Mn}}=$ 0.5 eV in comparison to $U_{\mathrm{Mn}}=$ 0, thus improving the agreement with the experiment. The shape also becomes symmetric with the shoulder at -1.8 eV for $U_{\mathrm{Mn}}=$ 0 almost absent for $U_{\mathrm{Mn}}=$ 0.5 eV, indicating better agreement with feature **B**. The other features (**A**, **C**-**E**) are largely unchanged. While for $U_{\mathrm{Mn}}=$ 1 eV there is no further improvement, for U>1 eV, the match with experiment is worsened as evident from a shift in feature **C** towards higher binding energy. For example, for $U_{\mathrm{Mn}}=$ 1.8 eV [25], feature **C** is shifted by 0.4 eV, in clear disagreement with the experiment. For $U_{\mathrm{Mn}}=$ 3.93 eV [26], feature **C** shifted further away to $X_3$ which is 1.3 eV away from the experimental position (see the red arrow). Moreover, feature **B** splits into two features $X_1$ and $X_2$ that are 0.5 eV apart. Also, feature **D** decreases in intensity with the appearance of a new weak feature $X_4$. None of the $X_n$ ($n=$ 2-4) features are observed experimentally. Turning to the comparison of saturation magnetization, we note that in literature, the experimental value of the saturation moment of stoichiometric $Ni_2MnGa$ in the martensite phase measured at ≤5K and fields up to 7 Tesla has been reported to be 4.04 – 4.27 $\mu_B$ [3, 27–29]. While 4.23$\mu_B$ was reported by Ooiwa *et al.* from M(H) measurement at 4.2 K and 6 Tesla, a value of 4.27$\mu_B$ has been extracted from the M(H) curve in Fig. 9 of Ref. [29] measured at 2 K and 7 Tesla. As shown in Table S6 of SM, the calculated total moment for $U_{\mathrm{Mn}}=$ 0 is 4.2 $\mu_B$ showing already a very good agreement. For $U_{\mathrm{Mn}} = 0.5$ eV, the moment is 4.28 $\mu_B$, a value that, although on the higher end, could be considered consistent with the experiment. However, for $U_{\mathrm{Mn}}=$ 1, the moment increases further to 4.35 $\mu_B$. For $U_{\mathrm{Mn}}=$ 1.8 eV suggested by Zeleney *et al.* [25] the moment is 4.47 $\mu_B$, whereas for $U_{\mathrm{Mn}}=$ 3.93 eV suggested by Koubsky *et al.* [26], the value is even larger, 4.68 $\mu_B$. Such large values of the moment (in disagreement with magnetization) and deviation in the shape of the valence band (in disagreement with HAXPES) demonstrate that the large $U_{\mathrm{Mn}}$ values suggested earlier [25, 26] are not correct; this is further discussed later. From the above discussions, we conclude that $U_{\mathrm{Mn}}$ of 0.5 eV seems to be a reasonable value from our GGA+U calculations, which improves the agreement with the HAXPES VB and gives a reasonable total moment compared to the experiment [3, 27–29]. Additionally, we have performed GGA+U calculations to examine whether the inclusion of $U_{\mathrm{Ni}}$ further improves the agreement with the experiment. However, in Fig. S10 of SM, we find that there is no improvement, rather the agreement is worsened with increasing $U_{\mathrm{Ni}}$ by (i) a shift of feature **B** and feature **C** towards higher binding energies (shown by red arrows) and (ii) a small but clear shift in feature **A** towards the

Fermi level, i.e., lower binding energies (compare the blue dashed vertical arrow with the red dashed arrow). The latter worsens the excellent agreement obtained in Fig. 3a with GGA. For $U_{\rm Ni}$= $U_{\rm Mn}$= 3 eV suggested by Jannovic et al. [24], we find that feature **B** is split into two components of nearly similar intensity ($X_2$ and $X_3$ separated by 0.3 eV) that are shifted from the experimental position by 0.5 eV. Feature **C** is also shifted by 0.9 eV to $X_4$. Feature **A** shifted towards lower binding energy by 0.2 eV to $X_1$. Finally, feature **D** splits into two weak features, $X_5$ and $X_6$, with a minimum at the experimental position of feature **D**. Thus, the theory features $X_m$, $m$= 1-6 are all in disagreement with the experimental features **A-D**. Moreover, as shown in Table S6, the total moment increases further with $U_{\rm Ni}$: for example, for $U_{\rm Ni}$= 1.0 (0.5) eV, the total moment is 4.36 (4.32) $\mu_B$. For larger values of $U_{\rm Ni}$ and $U_{\rm Mn}$ the moment increases further. Finally, for $U_{\rm Ni}$= $U_{\rm Mn}$= 3 eV, as suggested by Jannovic et al. [24], the moment is very large (4.81 $\mu_B$) in disagreement with the experiment. Thus, incorporation of $U_{\rm Ni}$ worsens the agreement with the experiment both for the VB and magnetic moment and so need not be considered. Thus, based on comparison with the HAXPS VB and the magnetic moment reported in literature, we conclude that GGA is sufficient to describe the electronic structure of $Ni_2MnGa$ since it provides a very good agreement with experiment. This is related to the use of the actual experimental structure [5, 6] for the DFT GGA calculation. We find that electron-electron correlation does not play a significant role in $Ni_2MnGa$ since a small value of a value of $U_{\rm Mn}$ of about 0.5 eV (with $U_{\rm Ni}$= 0) is suggested by our analysis that marginally improves the agreement with the HAXPES VB. Finally, we turn to how recent literature [24–26] arrived at such large values of $U$. Koubsky *et al* [26] reported $U_{\rm Mn}$ of 3.93 eV with $U_{\rm Ni}$= 0 by comparing the bulk modulus ($B$) from their GGA+U calculation with the experimental $B$ of 134 GPa from Seiner *et al.* [30]. However, Koubsky *et al.* disregarded another prior experimental work by Worgull *et al.* [31], where $B$ was reported to be 146 GPa, a result that was well reproduced (152 GPa) by a subsequent DFT calculation without invoking $U$ [32]. This shows that it is important for the theory groups to survey the whole gamut of experimental results in the literature. In particular, the complexity of the Ni-Mn-Ga system arises from the possible existence of non-stoichiometry that could alter the properties and the transition temperatures, as stated in the Introduction. In the present case, between Worgull *et al.* [31] (146 GPa) and Seiner *et al.* [30] (134 GPa), the main differences are in the $C_{11}$ value (152 GPa versus 140 GPa) that could arise from differences in the stoichiometry of their crystals. Moreover, as pointed out by Seiner et al. [30] this could also be related to a deviation from perfect alignment of the crystal. A subsequent theoretical paper [24] taking cue from Koubsky *et al.* [26] also compared their results with $B$= 134 GPa and arrived at $U_{\rm Mn} = U_{\rm Ni} = 3$ eV. Despite obtaining large values of moments for increasing $U$ and in particular for the suggested $U_{\rm Mn} = U_{\rm Ni} = 3$ eV [24], it was argued by the authors that the austenite phase moment from the experiment is large. This was concluded from values obtained by a linear extrapolation of the experimental $M^2$ versus $T^2$ data from literature ($M$ is magnetization) from above $M_s$ (i.e. 205-220 K) to zero temperature. Such linear extrapolation is a gross approximation with no theoretical basis and relies on phenomenological observation in a scarce data set [28]. Moreover, our present calculations show that the austenite phase total moment (4.04 $\mu_B$) is actually smaller compared to the martensite phase (4.20 $\mu_B$) as shown in Table S6. This remains so for non-zero $U_{\rm Mn}$ and $U_{\rm Ni}$, except at large values of $U$ the austenite phase moment is marginally larger (last two rows of Table S6). This refutes the misleading impression conveyed in Fig. 1c of Ref. 24 by considering experimental magnetization values in the literature that the austenite phase has a larger "experimental" saturation moment compared to the experimental value in the martensite phase. Thus, based on questionable values of the "experimental" saturation moment in austenite phase obtained by extrapolation, these authors arrived at a large $U$. To obtain correct results, the martensite phase moment in the experimental literature should be compared with the results of DFT theory using the actual structure of the martensite phase, as has been done in our present work. In another work, Zeleny *et al.* [25] reported a $U_{\rm Mn}$ of 1.8 eV ($U_{\rm Ni}$= 0) since for this $U$ they obtained an almost tetragonal structure with $c/a = 0.925$ for the martensite phase. A fundamental flaw here in the calculation for the martensite phase [24, 25] is that the calculations were conducted using either non-modulated structure or model structures derived from the nano-twin model [20] that are not the correct structures for stoichiometric $Ni_2MnGa$ in the martensite phase [4–6].

## V. NOTE D

*Effect of Disorder* – Although anti-site disorder is not reported to be present in stoichiometric $Ni_2MnGa$ [4–6], for the sake of completeness, we have conducted theoretical investigations to explore the possible effects of anti-site disorder. We have introduced anti-site disorder in the MDL-S structure by randomly swapping one Mn atom with (i) Ni and (ii) Ga atoms. Thus, 7% of the Mn atoms contribute to anti-site disorder (there are 14 Mn atoms in the 56 atom unit cell). The calculated spin-polarized DOS for the two disordered structures (Mn-Ga swap and Mn-Ni swap) show that the position of all the features in the DOS remains unchanged (see Fig. S11 of SM). However, as is expected for disorder, a small broadening of the features is observed, as was also shown by our earlier works on related ternary intermetallic compounds with anti-site disorder [14, 33].

Table S1. Spacegroup, cell parameters (a = b = c in Å; $\alpha = \beta = \gamma$ in degrees), site symmetries, fractional atomic positions ($x$, $y$, $z$) of the cubic $L2_1$ austenite phase.

| Spacegroup | Cell Parameters | | Atom | Site Symmetries | Fractional Coordinates | | |
|---|---|---|---|---|---|---|---|
| | a | $\alpha$ | | | x | y | z |
| $Fm\bar{3}m$ | 5.81 | 90 | Ga | 4a | 0.00 | 0.00 | 0.00 |
| | | | Mn | 4b | 0.50 | 0.50 | 0.5 |
| | | | Ni | 8c | 0.25 | 0.25 | 0.25 |

Table S2. Spacegroup, cell parameters (a, b, c in Å, $\alpha = \beta = \gamma$ in degrees), site symmetries, fractional atomic positions ($x$, $y$, $z$) for the 7M modulated structure of the martensite phase of $Ni_2MnGa$ as given by Brown *et al.* [4].

| Spacegroup | Cell Parameters | | | | Atom | Site Symmetries | Fractional Coordinates | | |
|---|---|---|---|---|---|---|---|---|---|
| | a | b | c | $\alpha$ | | | x | y | z |
| Pnnm | 4.215 | 29.302 | 5.557 | 90 | Ga1(2) | 2b | 0.000 | 0.00 | 0.50 |
| | | | | | Ga2(4) | 4g | 0.009 | 1/7 | 0.50 |
| | | | | | Ga3 (4) | 4g | 0.026 | 2/7 | 0.50 |
| | | | | | Ga4 (4) | 4g | 0.062 | 3/7 | 0.50 |
| | | | | | Mn1 (2) | 2a | 0.000 | 0.00 | 0.00 |
| | | | | | Mn2 (4) | 4g | 0.041 | 1/7 | 0.50 |
| | | | | | Mn3 (4) | 4g | -0.070 | 2/7 | 0.050 |
| | | | | | Mn4 (4) | 4g | 0.072 | 3/7 | 0.50 |
| | | | | | Ni1 (4) | 4f | 0.500 | 0 | 0.25 |
| | | | | | Ni2 (8) | 8h | 0.476 | 1/7 | 0.25 |
| | | | | | Ni3(8) | 8h | 0.549 | 2/7 | 0.25 |
| | | | | | Ni4(8) | 8h | 0.433 | 3/7 | 0.25 |

Table S3. Spacegroup, cell parameters (a, b, c in Å, $\alpha = \beta = \gamma$ in degrees), site symmetries, fractional atomic positions ($x$, $y$, $z$) for the 7M modulated structure of the martensite phase of $Ni_2MnGa$ as given by Righi *et al.* [5].

| Spacegroup | Cell Parameters | | | | Atom | Site Symmetries | Fractional Coordinates | | |
|---|---|---|---|---|---|---|---|---|---|
| | a | b | c | $\alpha$ | | | x | y | z |
| Pnnm | 4.219 | 29.332 | 5.554 | 90 | Ga1(2) | 2b | 0.0000 | 0.00 | 0.50 |
| | | | | | Ga2(4) | 4g | 0.0298 | 1/7 | 0.50 |
| | | | | | Ga3 (4) | 4g | 0.9450 | 2/7 | 0.50 |
| | | | | | Ga4 (4) | 4g | 0.0669 | 3/7 | 0.50 |
| | | | | | Mn1 (2) | 2a | 0.0000 | 0.00 | 0.00 |
| | | | | | Mn2 (4) | 4g | 0.0289 | 1/7 | 0.50 |
| | | | | | Mn3 (4) | 4g | 0.0520 | 2/7 | 0.50 |
| | | | | | Mn4 (4) | 4g | 0.0649 | 3/7 | 0.50 |
| | | | | | Ni1(4) | 4f | 0.5000 | 0 | 0.25 |
| | | | | | Ni2 (8) | 8h | 0.5314 | 1/7 | 0.25 |
| | | | | | Ni3(8) | 8h | 0.4434 | 2/7 | 0.25 |
| | | | | | Ni4(8) | 8h | 0.5705 | 3/7 | 0.25 |

Table S4. Symmetry, cell parameters (a, b, c in Å, $\alpha = \beta = \gamma$ in degrees), fractional atomic positions ($x$, $y$, $z$) for the 7M modulated structure of the martensite phase of $Ni_2MnGa$ as given by Singh *et al.* [6].

| Symmetry | Cell Parameters | | | | Atom | Site Symmetries | Fractional Coordinates | | |
|---|---|---|---|---|---|---|---|---|---|
| | a | b | c | $\alpha$ | | | x | y | z |
| Pnnm | 4.219 | 29.313 | 5.547 | 90 | Ga1(2) | 2b | 0.0000 | 0.00 | 0.50 |
| | | | | | Ga2(4) | 4g | 0.0230 | 1/7 | 0.50 |
| | | | | | Ga3 (4) | 4g | 0.9510 | 2/7 | 0.50 |
| | | | | | Ga4 (4) | 4g | 0.0680 | 3/7 | 0.50 |
| | | | | | Mn1 (2) | 2a | 0.0000 | 0.00 | 0.00 |
| | | | | | Mn2 (4) | 4g | 0.0280 | 1/7 | 0.50 |
| | | | | | Mn3 (4) | 4g | 0.9480 | 2/7 | 0.50 |
| | | | | | Mn4 (4) | 4g | 0.0649 | 3/7 | 0.50 |
| | | | | | Ni1(4) | 4f | 0.5000 | 0 | 0.25 |
| | | | | | Ni2 (8) | 8h | 0.5230 | 1/7 | 0.25 |
| | | | | | Ni3(8) | 8h | 0.4540 | 2/7 | 0.25 |
| | | | | | Ni4(8) | 8h | 0.5640 | 3/7 | 0.25 |

Table S5. Spacegroup, cell parameters (a, b, c in Å, $\alpha$, $\beta$, $\gamma$ in degrees), fractional atomic positions ($x$, $y$, $z$) of the nanotwin (NTN-K) structure of the martensite phase [20].

| Spacegroup | Cell Parameters | | | | | | Atom | Fractional Coordinates | | |
|---|---|---|---|---|---|---|---|---|---|---|
| | a | b | c | $\alpha$ | $\beta$ | $\gamma$ | | x | y | z |
| P1 | 4.292 | 29.535 | 5.365 | 90 | 90 | 84.2 | Ga1 | 0.9601 | 0.0001 | 0.0000 |
| | | | | | | | Ga2 (2) | 0.5108 | 0.0710 | 0.5000 |
| | | | | | | | Ga3 (2) | 0.0716 | 0.1431 | 0.0000 |
| | | | | | | | Ga4 (2) | 0.6289 | 0.2140 | 0.5000 |
| | | | | | | | Ga5(2) | 0.1897 | 0.2861 | 0.0000 |
| | | | | | | | Ga6 (2) | 0.7402 | 0.3570 | 0.5000 |
| | | | | | | | Ga7 (2) | 0.1001 | 0.4286 | 0.0000 |
| | | | | | | | Mn1 (2) | 0.9601 | 0.0001 | 0.5000 |
| | | | | | | | Mn2 (2) | 0.5108 | 0.0710 | 0.0000 |
| | | | | | | | Mn3 (2) | 0.0716 | 0.1431 | 0.5000 |
| | | | | | | | Mn4 (2) | 0.6289 | 0.2140 | 0.0000 |
| | | | | | | | Mn5 (2) | 0.1897 | 0.2861 | 0.5000 |
| | | | | | | | Mn6 (2) | 0.7402 | 0.3570 | 0.0000 |
| | | | | | | | Mn7(2) | 0.1001 | 0.4286 | 0.5000 |
| | | | | | | | Ni1 (4) | 0.4514 | 0.0000 | 0.2503 |
| | | | | | | | Ni2(4) | 0.0104 | 0.0721 | 0.2498 |
| | | | | | | | Ni3(4) | 0.5706 | 0.3570 | 0.2501 |
| | | | | | | | Ni4(4) | 0.1299 | 0.4286 | 0.7498 |
| | | | | | | | Ni5(4) | 0.6902 | 0.2850 | 0.2502 |
| | | | | | | | Ni6 (4) | 0.2489 | 0.3571 | 0.2497 |
| | | | | | | | Ni7 (4) | 0.6001 | 0.4285 | 0.2500 |

Table S6. Total and atom projected magnetic moments ($\mu_B$ /f.u.) in the MDL-S modulated martensite and austenite phases of $Ni_2MnGa$ using the GGA+U exchange correlation functional.

| Coulomb correlation U (in eV) | Martensite phase | | | | Austenite phase | | | |
|---|---|---|---|---|---|---|---|---|
| $U_{Mn}$,$U_{Ni}$ | Total | Ni | Mn | Ga | Total | Ni | Mn | Ga |
| 0.0, 0.0 | 4.20 | 0.41 | 3.37 | -0.04 | 4.04 | 0.35 | 3.27 | -0.04 |
| 0.5, 0.0 | 4.28 | 0.42 | 3.52 | -0.04 | 4.14 | 0.34 | 3.40 | -0.04 |
| 1.0, 0.0 | 4.35 | 0.43 | 3.64 | -0.04 | 4.22 | 0.33 | 3.51 | -0.05 |
| 1.8, 0.0 [25] | 4.47 | 0.42 | 3.80 | -0.04 | 4.34 | 0.30 | 3.67 | -0.05 |
| 3, 0.0 | 4.60 | 0.33 | 3.98 | -0.04 | 4.48 | 0.27 | 3.86 | -0.05 |
| 3.93, 0.0 [26] | 4.68 | 0.30 | 4.12 | -0.04 | 4.56 | 0.24 | 3.99 | -0.04 |
| 0.5, 0.5 | 4.32 | 0.42 | 3.51 | -0.08 | 4.18 | 0.36 | 3.40 | -0.05 |
| 0.5, 1.0 | 4.36 | 0.45 | 3.51 | -0.08 | 4.23 | 0.38 | 3.41 | -0.05 |
| 1.0, 0.5 | 4.39 | 0.42 | 3.64 | -0.04 | 4.27 | 0.35 | 3.51 | -0.04 |
| 1.0, 1.0 | 4.43 | 0.45 | 3.65 | -0.04 | 4.32 | 0.37 | 3.52 | -0.05 |
| 1.8, 1.0 | 4.55 | 0.42 | 3.81 | -0.04 | 4.44 | 0.35 | 3.68 | -0.05 |
| 1.8, 2.0 | 4.62 | 0.46 | 3.80 | -0.04 | 4.56 | 0.41 | 3.70 | -0.05 |
| 1.8, 3.0 | 4.69 | 0.51 | 3.80 | -0.04 | 4.72 | 0.48 | 3.71 | -0.05 |
| 3.0, 3.0 [24] | 4.81 | 0.47 | 4.02 | -0.05 | 4.86 | 0.45 | 3.90 | -0.04 |

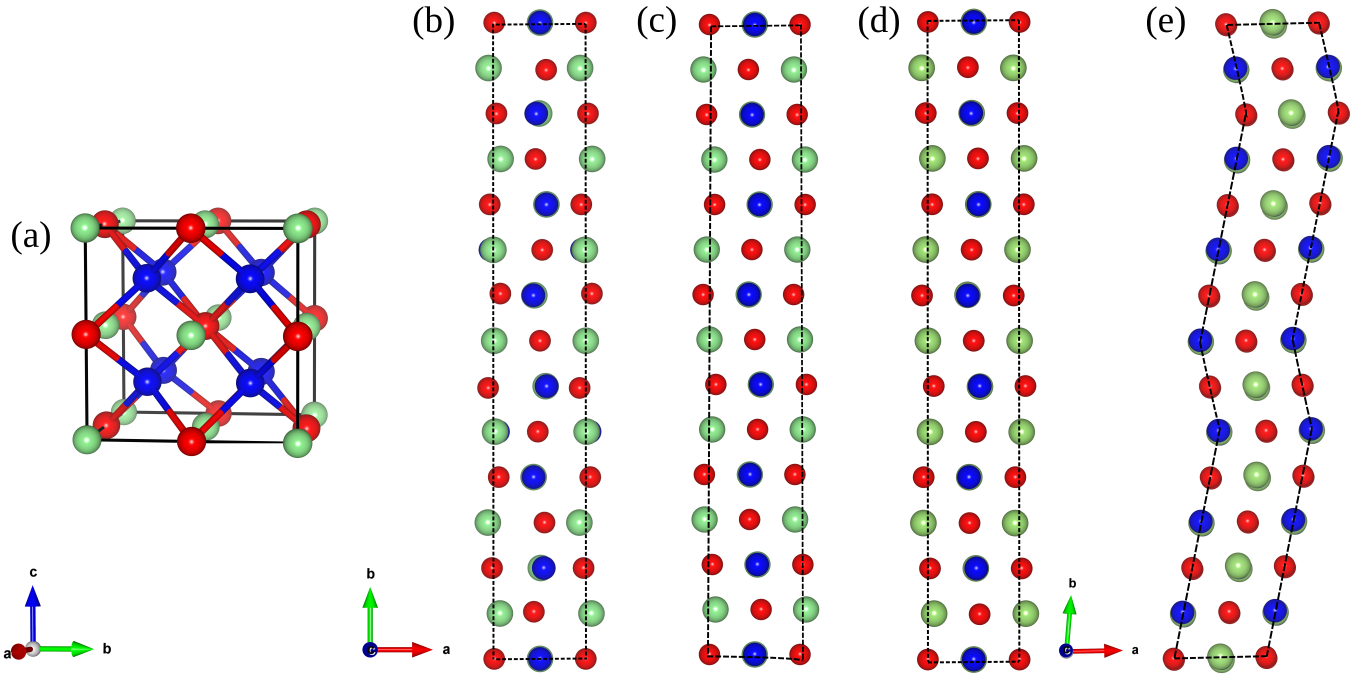


Figure S1. The structure of the (a) austenite phase of $Ni_2MnGa$ compared with the experimental modulated structures in the martensite phase: (b) MDL-B [4], (c) MDL-R [5], (d) MDL-S [6], and (e) the relaxed NTN-K structure [20]. Red, green and blue spheres correspond to Mn, Ga and Ni atoms, respectively. The structures have been obtained from the structural parameters presented in Tables S1-S5, using the software VESTA [34].

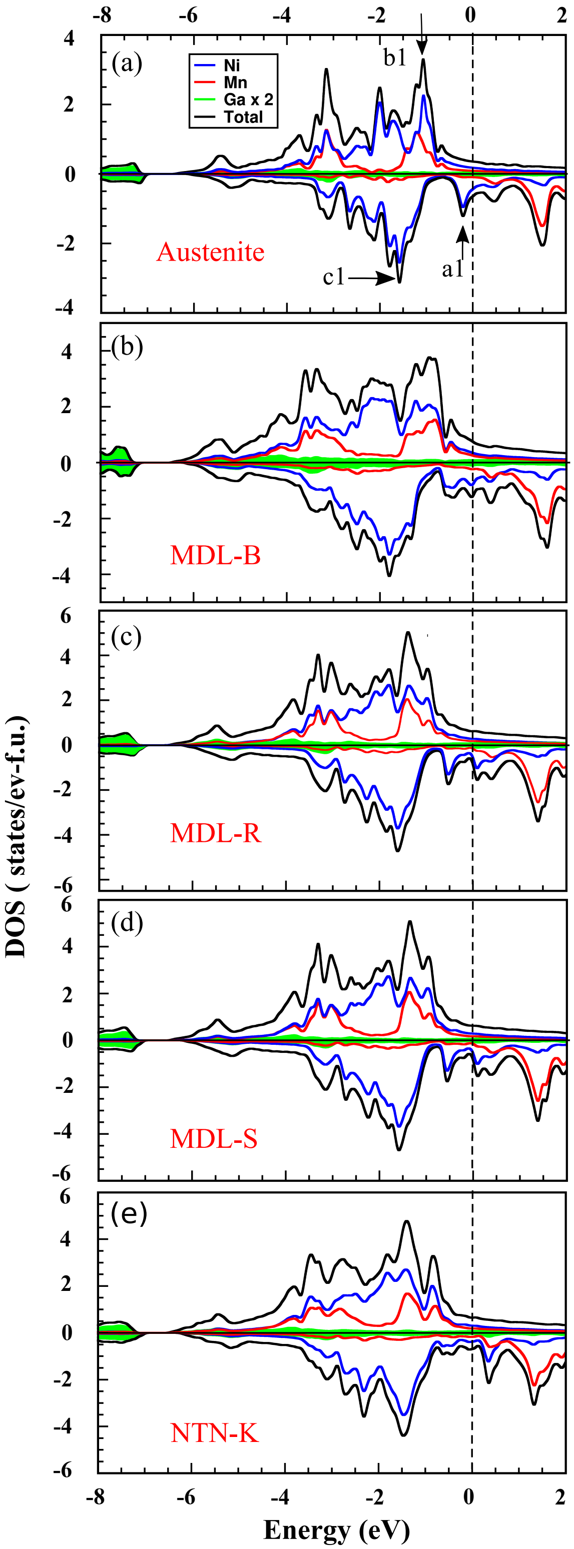


Figure S2. Spin-resolved majority and minority spin DOS and atom projected PDOS of $Ni_2MnGa$ for (a) austenite and martensite phase: (b) MDL-B, (c) MDL-R, (d) MDL-S, and (e) NTN-K structures. For better visualization, the DOS of Ga atom has been multiplied by a factor of 2. The $E_F$ is set to zero for all the cases.

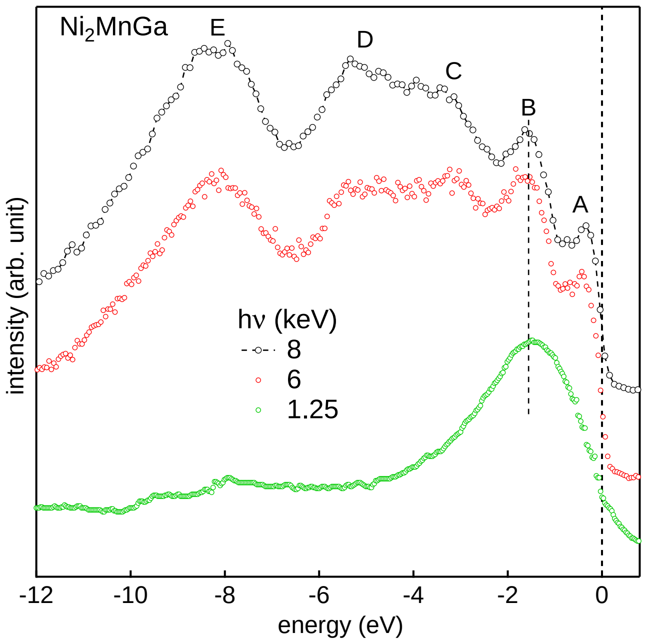


Figure S3. The experimental HAXPES VB spectra of $Ni_2MnGa$ in the austenite phase taken with 8 and 6 keV compared with the XPS spectrum taken with 1.25 keV.

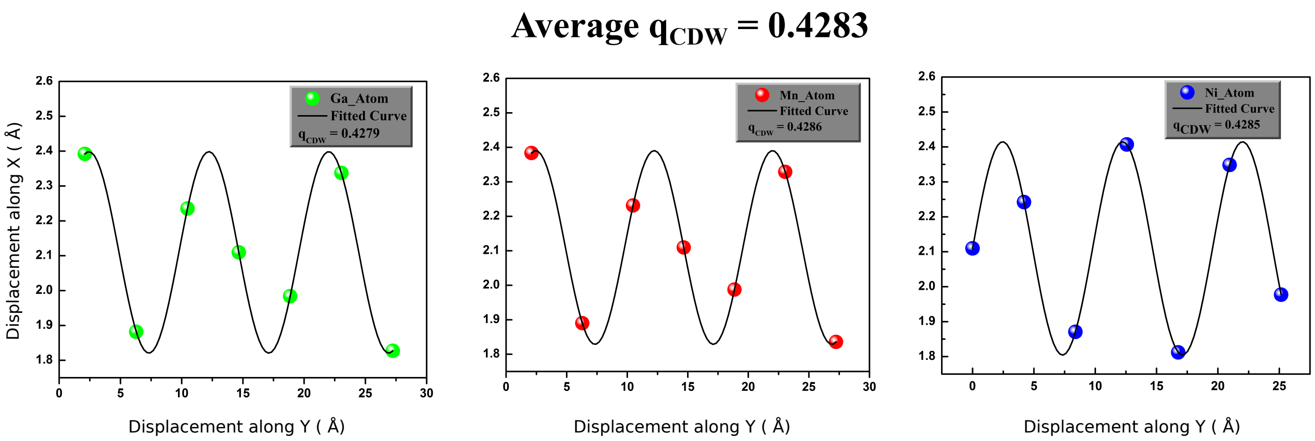


Figure S4. Modulations for the Ga, Mn and Ni atoms in the Pnnm 7-fold modulated structure of $Ni_2MnGa$ in the martensite phase, as given by Righi *et al* [5]. The solid curves are the fitted ones for the CDW displacements as a function of displacement along Y direction. The average $q_{CDW}$ value is also mentioned (in bold) at the top of the figure.

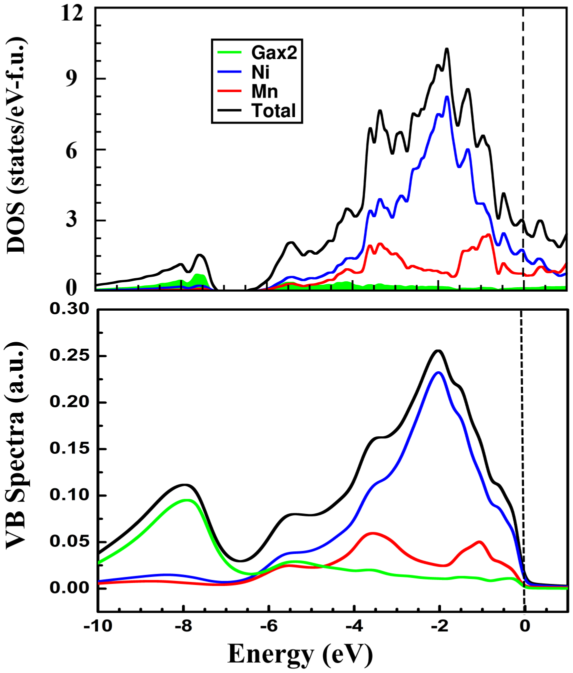


Figure S5. Spin-integrated total DOS and atom projected PDOS of the 7-fold modulated MDL-B structure [4] for the martensite phase of $Ni_2MnGa$ (top panel) and the calculated valence band spectrum with atom projected partial components (bottom panel). The $E_F$ has been set to zero and for better visualization, the DOS of the Ga atom has been multiplied by a factor of 2.

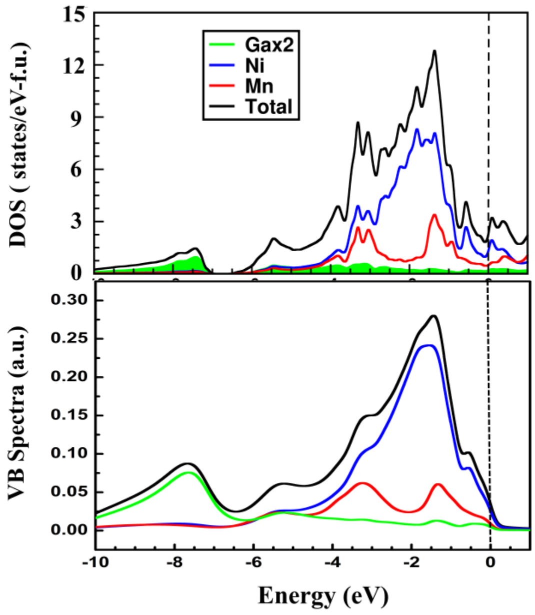


Figure S6. Spin-integrated total DOS and atom projected PDOS of the 7-fold modulated MDL-R structure [5] for the martensite phase of $Ni_2MnGa$ (top panel) and the calculated valence band spectrum with atom projected partial components (bottom panel). $E_F$ has been set to zero. For better visualization, the DOS of the Ga atom has been multiplied by a factor of 2.

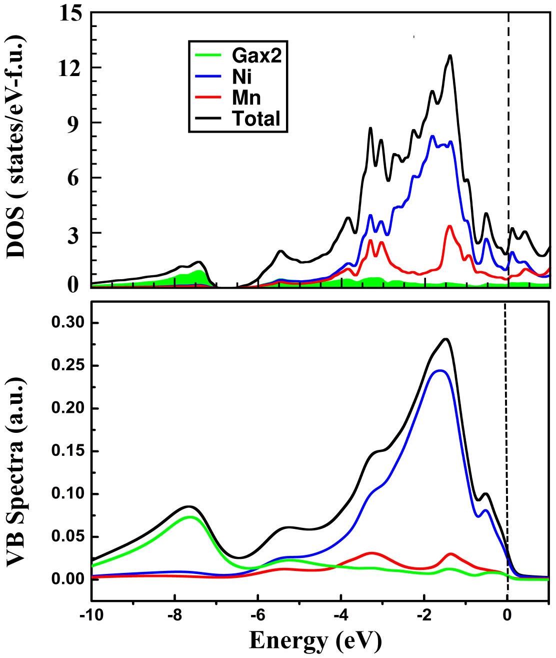


Figure S7. Spin-integrated total DOS and atom projected PDOS of the 7-fold modulated MDL-S structure [6] for the martensite phase of $Ni_2MnGa$ (top panel) and the calculated valence band spectrum with atom projected partial components (bottom panel). $E_F$ is set to zero. For better visualization, the DOS of the Ga atom has been multiplied by a factor of 2.

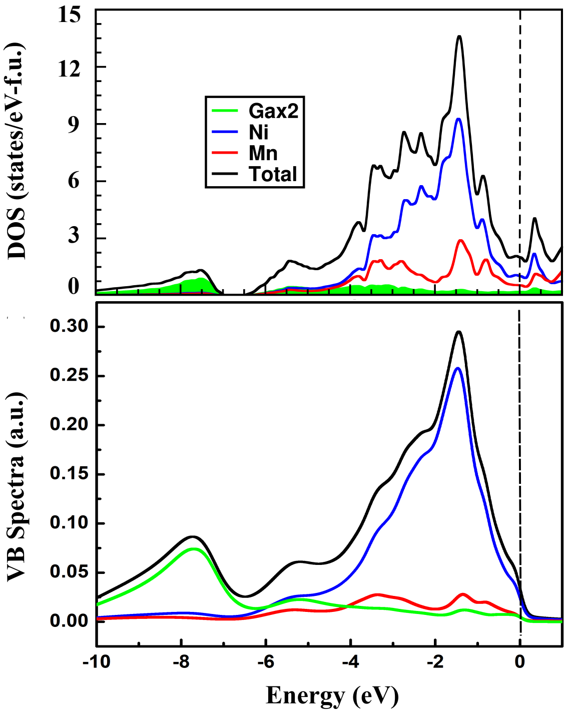


Figure S8. Spin-integrated total DOS and atom projected PDOS of the nanotwin NTN-K structure [20] in the martensite phase of $Ni_2MnGa$ (top panel) and the calculated valence band spectrum with atom projected partial components (bottom panel). $E_F$ has been set to zero. For better visualization, the DOS of the Ga atom has been multiplied by a factor of 2.

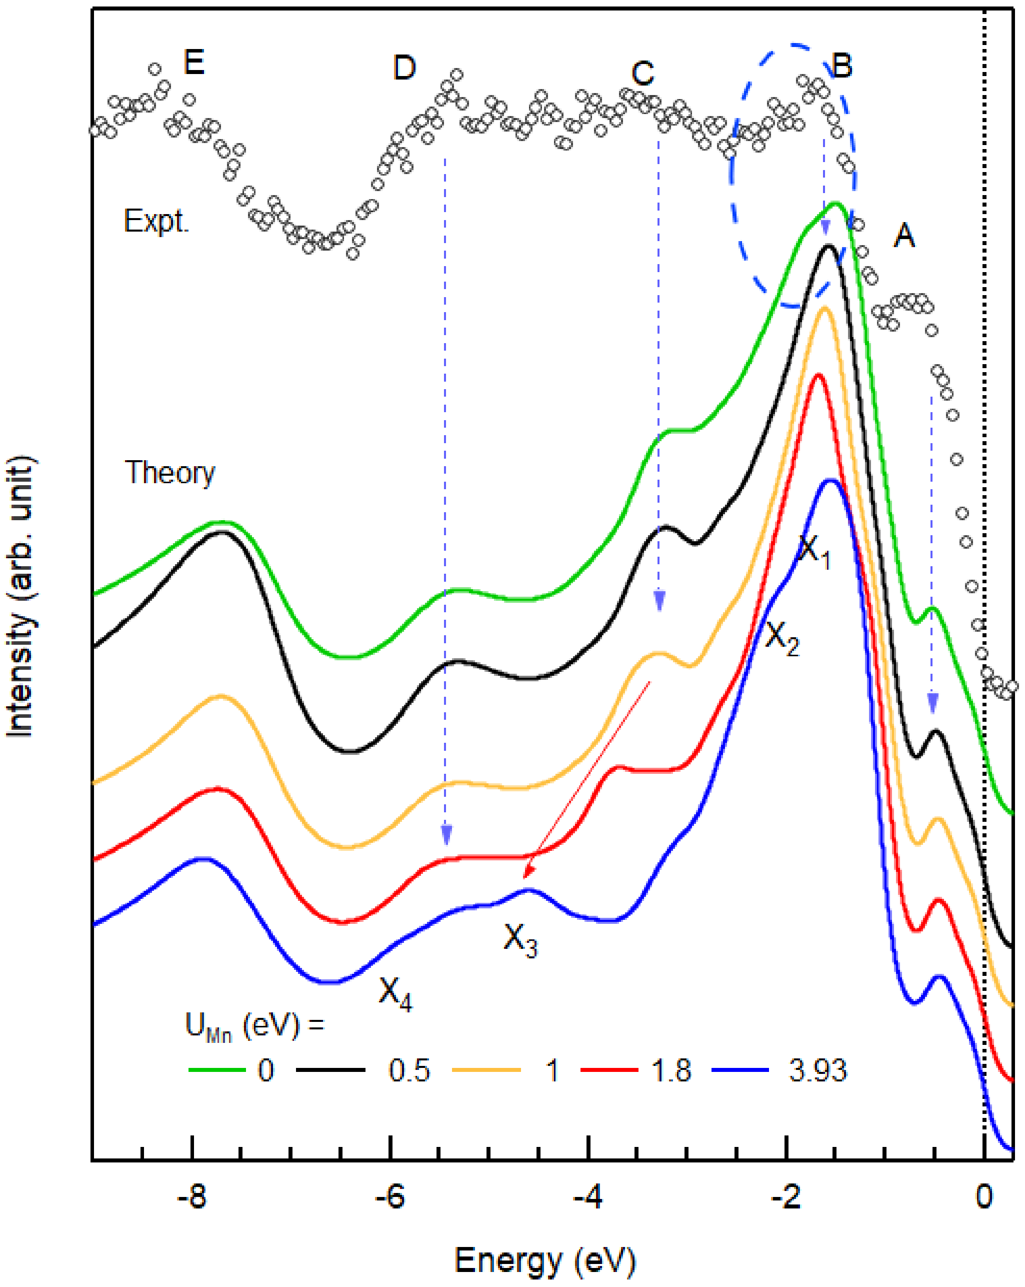


Figure S9. The theoretical VB spectra calculated for 7-fold modulated MDL-S martensite structure with $0 \leq U_{Mn} \leq 3.93$ eV values compared with the experimental VB spectrum in the martensite phase. The zero of the horizontal energy scale corresponds to the Fermi level. The spectra have been staggered along the vertical axis.

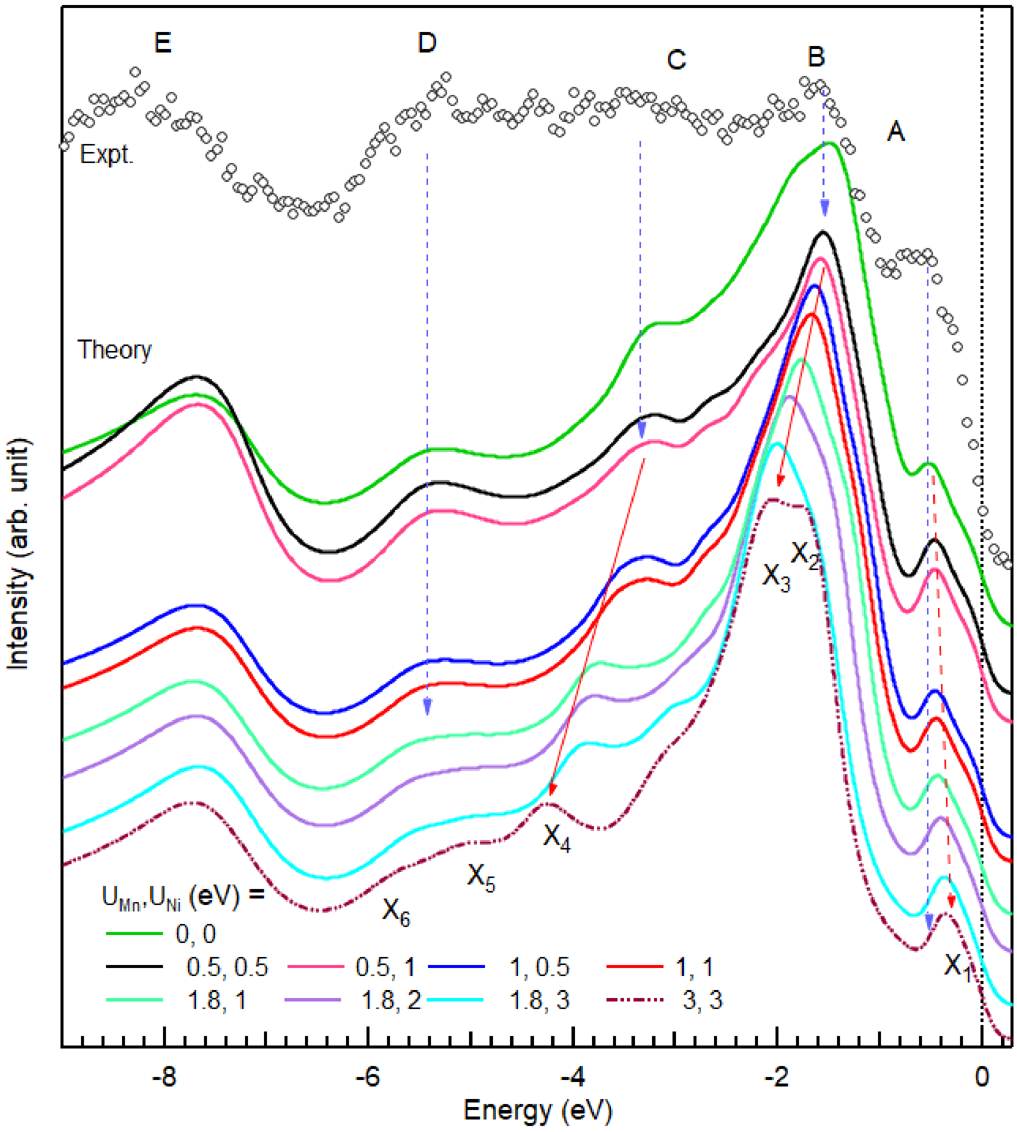


Figure S10. The theoretical VB spectra calculated for 7-fold modulated MDL-S martensite structure with $0 \leq U_{Mn}$, $U_{Ni} \leq$ 3 eV values compared with the experimental VB spectrum in the martensite phase. The zero of the horizontal energy scale corresponds to the Fermi level. The spectra have been staggered along the vertical axis.

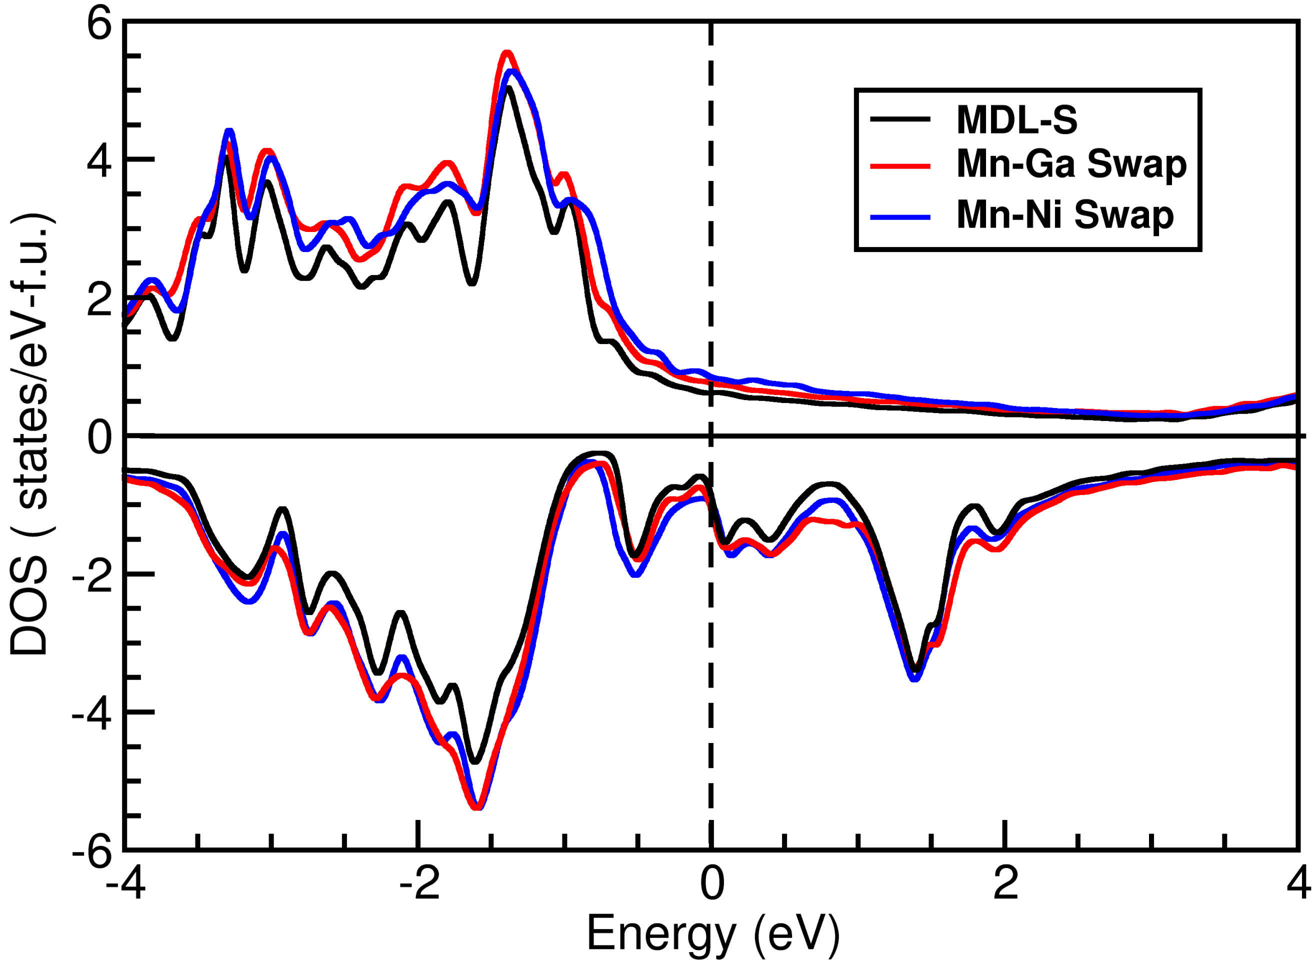


Figure S11. Spin-polarized density of states of MDL-S structure compared with two structures where anti-site disorder has been introduced by randomly swapping (i) one Mn atom with one Ni atom (Mn-Ni swap) and (ii) one Mn atom with one Ga atom (Mn-Ga swap) in the 56 atom unit cell.

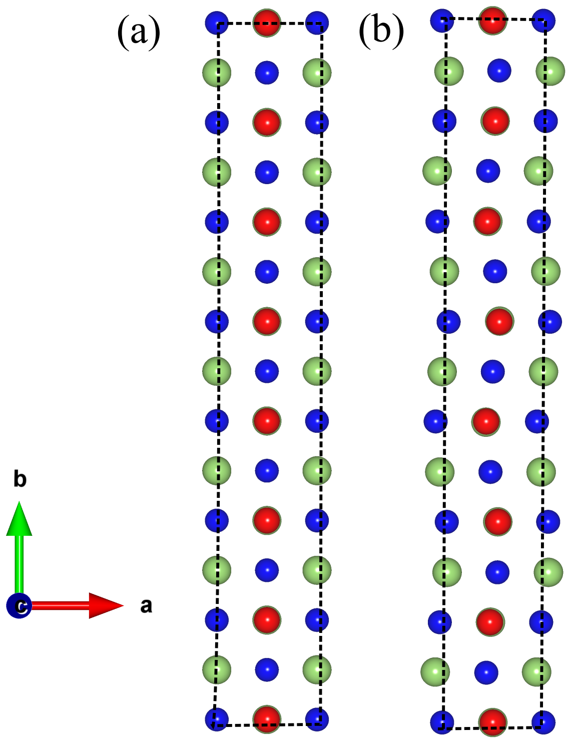


Figure S12. The non-modulated martensite structure (NMDL-S) on the left side is compared with the MDL-S structure on the right side. The former has the same lattice constants as the latter, but the amplitude of modulation set to zero.

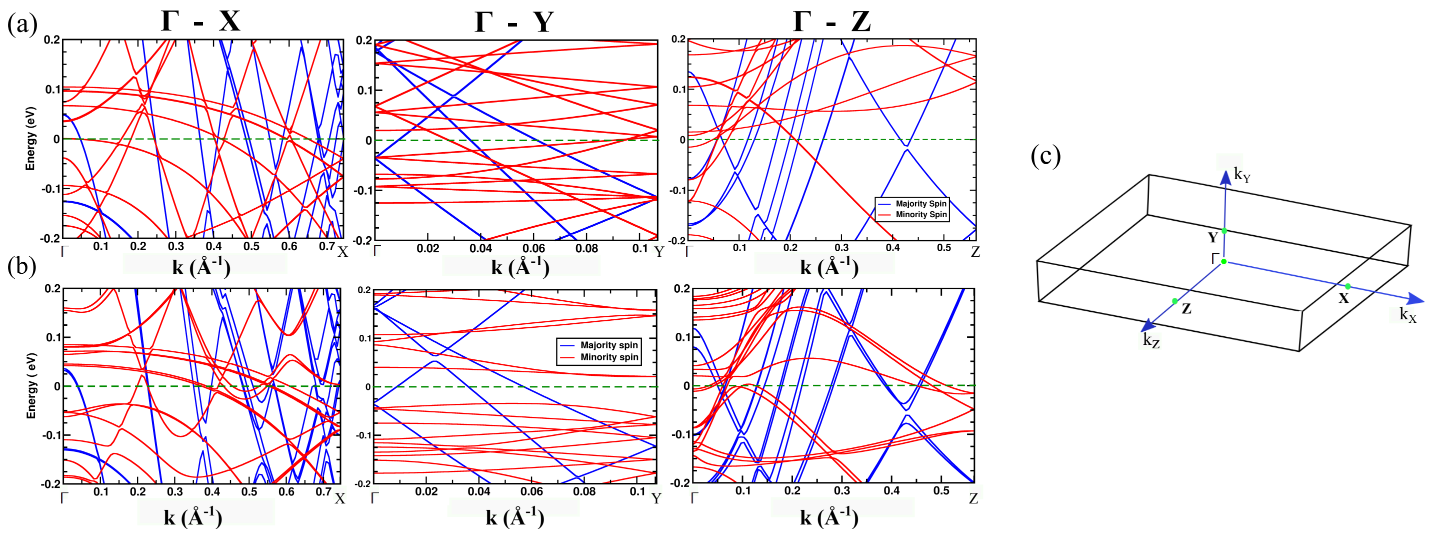


Figure S13. Calculated band structure along the high symmetry directions $\Gamma X$, $\Gamma Y$, and ΓZ for (a) non-Modulated martensite structure (NMDL-S) and (b) MDL-S structure. (c) The Brillouin zone along with the high symmetry points.

[1] G. Kresse and J. Furthmüller, Phys. Rev. B **54**, 11169 (1996); G. Kresse and D. Joubert, Phys. Rev. B **59**, 1758 (1999).

[2] J. P. Perdew, K. Burke, and M. Ernzerhof, Phys. Rev. Lett. **77**, 3865 (1996).

[3] P. J. Webster, K. R. A. Ziebeck, S. L. Town, and M. S. Peak, Philos. Mag. B **49**, 295 (1984).

[4] P. J. Brown, J. Crangle, T. Kanomata, M. Matsumoto, K. -U. Neumann, B. Ouladdiaf, and K. R. A. Ziebeck, J. Phys. Cond. Mater. **14**, 10159 (2002).

[5] L. Righi, F. Albertini, G. Calestani, L. Pareti, A. Paoluzi, C. Ritter, P. A. Algarabel, L. Morellon, and M. R. Ibarra, J. Solid State Chem. **179**, 3525 (2006).

[6] S. Singh, V. Petricek, P. Rajput, A. H. Hill, E. Suard, S. R. Barman, and D. Pandey, Phys. Rev. B **90**, 014109 (2014).

[7] S. Singh, J. Bednarcik, S. R. Barman, C. Felser, and D. Pandey, Phys. Rev. B **92**, 054112 (2015).

[8] H.J. Monkhorst and J.D. Pack, Phys. Rev. B **13**, 5188 (1976).

[9] A. Gloskovskii, G. Stryganyuk, G. H. Fecher, C. Felser, S. Thiess, H. Schulz-Ritter, W. Drube, G. Berner, M. Sing, R. Claessen, and M. Yamamoto, J. Electron Spectrosc. Relat. Phenom. **185**, 47 (2012).

[10] D. L. Schlagel, Y. L.Wu, W. Zhang, and T. A. Lograsso, J. Alloys Compd. **312**, 77 (2000).

[11] S.W. D′Souza, A. Rai, J. Nayak, M. Maniraj, R. S. Dhaka, S. R. Barman, D. L. Schlagel, T. A. Lograsso, and A. Chakrabarti, Phys. Rev. B **85**, 085123 (2012).

[12] S. W. D′Souza, R. S. Dhaka, A. Rai, M. Maniraj, J. Nayak, S. Singh, D. L. Schlagel, T. A. Lograsso, A. Chakrabarti, and S. R. Barman, Mater. Sci. Forum **684**, 215 (2011).

[13] R. S. Dhaka, S. W. D′Souza, M. Maniraj, A. Chakrabarti, D. L. Schlagel, T. A. Lograsso, and S. R. Barman, Surf. Sci. **603** 1999 (2009 ).

[14] P. Sadhukhan, S. W. D′Souza, V. K. Singh, R. S. Dhaka, A. Gloskovskii, S. K. Dhar, P. Raychaudhuri, A. Chainani, A. Chakrabarti, and S. R. Barman, Phys. Rev. B **99**, 035102 (2019).

[15] M. B. Trzhaskovskaya and V. G. Yarzhemsky, Atomic Data Nucl. Data Tables, **119**, 99 (2018).

[16] S. R. Barman and D. D. Sarma, Phys. Rev. B **51**, 4007 (1995).

[17] D. A. Shirley, Phys. Rev. B **5**, 4709 (1972).

[18] A. Chakrabarti, M. Siewert, T. Roy, K. Mondal, A. Banerjee, M. E. Gruner, and P. Entel, Phys. Rev. B **88**, 174116 (2013); A. T. Zayak, P. Entel, K. M. Rabe, W. A. Adeagbo, and M. Acet, Phys. Rev. B **72**, 054113 (2005).

[19] A. Chakrabarti, C. Biswas, S. Banik, R. S. Dhaka, A. K. Shukla, and S. R. Barman, Phys. Rev. B **72**, 073103 (2005).

[20] S. Kaufmann, U. K. Rößler, O. Heczko, M. Wuttig, J. Buschbeck, L. Schultz, and S. Fähler, Phys. Rev. Lett. **104**, 145702 (2010).

[21] M. E. Gruner, R. Niemann, P. Entel, R. Pentcheva, U. K. Roessler, K. Nielsch, and S. Fähler, Sci. Rep. **8**, 8489 (2018).

[22] S. Fujii, S. Ishida, and S. Asano, J. Phy. Soc. Japan **58**, 3657 (1989).

[23] S. R. Barman, S. Banik, and A. Chakrabarti, Phys. Rev. B **72**, 184410 (2005).

[24] J. Janovec, M. Zeleny, O. Heczko, A. Ayuela, Sci Rep **12**, 20577 (2022).

[25] M. Zeleny, P. Sedlak, O. Heczko, H. Seiner, P. Vertat, M. Obata, T. Kotani, T. Oda, L. Straka, Mater. Des. **209**, 109917 (2021).

[26] T. Koubský, P. Sedlák, H. Seiner, J. Fojtíková, M. Obatac, T. Odac and L. Kalvoda, Acta Phys. Pol. A **134**, 2019 (2018).

[27] U. Devarajan, S. E. Muthu, S. Arumugam, S. Singh, and S. R. Barman, J. Appl. Phys. **114**, 053906 (2013).

[28] K. Ooiwa, K. Endo, and A. Shinogi, J. Magn. Magn. Mater. **104–107**, 2011 (1992).

[29] S. Singh, S. W. D′Souza, J. Nayak, L. Caron, E. Suard, S. Chadov, and C. Felser, Phys. Rev. B **93**, 134102 (2016).

[30] H. Seineř, O. Heczko, P. Sedlák, L. Bodnárová, M. Novotný, J. Kopecek̆ , M. Landa, J. Alloy. Comps. **577S**, S131 (2013).

[31] J. Worgull, E. Petti, and J. Trivisonno, Phys. Rev. B **54**, 15695 (1996).

[32] Q.-M. Hu, C.-M. Li, R. Yang, S. E. Kulkova, D. I. Bazhanov, B. Johansson, L. Vitos, Phys. Rev. B **79**, 144112 (2009).

[33] S. W. D′Souza, T. Roy, S. R. Barman and A. Chakrabarti, J. Phys. Condens. Matter **26**, 506001 (2014).

[34] K. Momma and F. Izumi, J. Appl. Crystallogr. **44**, 1272 (2011).
